# Supplementary material for: A constraint-based approach to granular dispersion rheology
Source: arXiv:1807.11356 ancillary file (2018-07-30)
Supplement: Supplementary file 1 [file constraints_arXiv_SI_resubmission.pdf]

# Supplementary Information: A constraint-based approach to granular dispersion rheology

B. M. Guy, J. A. Richards, D. J. M. Hodgson, E. Blanco, and W. C. K. Poon

*SUPA, School of Physics and Astronomy,*

*The University of Edinburgh, King's Buildings,*

*Peter Guthrie Tait Road, Edinburgh, EH9 3FD, United Kingdom*

(Dated: July 30, 2018)

In §S1, we demonstrate the effect of varying $\alpha/\beta$ at fixed $\sigma_{\mathrm{A}}/\sigma_{\mathrm{B}}$ for class 3b flow curves. In §S2, we present the class 3c flow curves predicted by our model. In §S3, we examine the relationship between different classes by systematically varying $\sigma_{\mathrm{A}}/\sigma_{\mathrm{B}}$. In §S4 A, we plot jamming phase diagrams for the cases of class 3a not considered in the main text and include further information on our comparison with experimental data in Fig. 3. In §S4 B, we plot an example jamming phase diagram for class 3b. In §S5, we compare the $\sigma$-$\phi$ phase diagrams for classes 1 and 3a presented in the main text. We also comment on the utility of our approach when experimental data is restricted to a narrow $\sigma$-window.

## S1. SENSITIVITY OF CLASS 3B RHEOLOGY TO $\alpha/\beta$

In the main text, we showed that the location (in stress terms) and height of the viscosity peak in the class 3b regime were sensitive to small changes in $\sigma_{\rm A}/\sigma_{\rm B}$ at fixed $\alpha/\beta$. The peak is similarly sensitive to changes in $\alpha/\beta$ at fixed $\sigma_{\rm A}/\sigma_{\rm B}$, Fig. S1. At $\sigma_{\rm A}/\sigma_{\rm B} = 0.45$ ($\phi = 0.69\phi_{\rm AB}$), increasing $\alpha/\beta$ by factor of three from 0.6 to 1.7, Fig. S1(b), gives rise to an order-of-magnitude variation in peak height, Fig. S1(a).

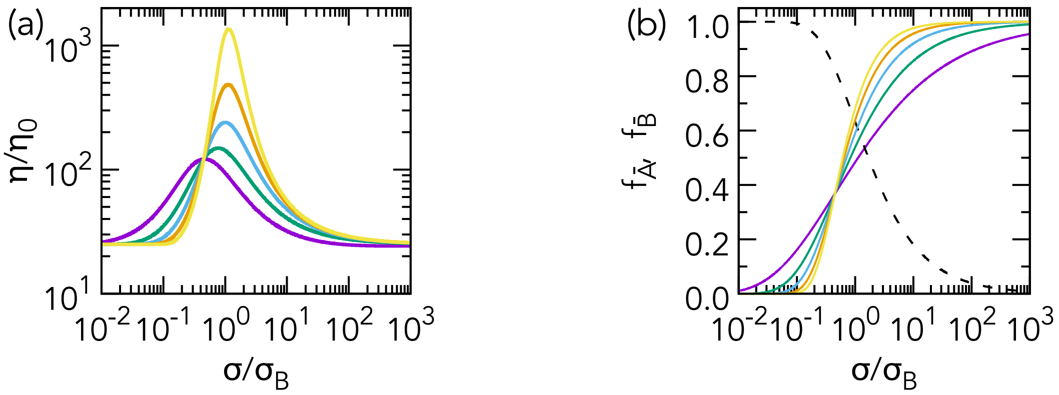


FIG. S1. Effect of varying $\alpha/\beta$ on class 3b phenomenology. Jamming points and volume fraction same as main text: $\phi_{\bar{\rm A}{\rm B}} = \phi_{{\rm A}\bar{\rm B}} = 0.86\phi_{\rm AB}$ and $\phi_{\bar{\rm A}\bar{\rm B}} = 0.47\phi_{\rm AB}$, and $\phi = 0.69\phi_{\rm AB}$. (a) $\eta/\eta_0$ versus $\sigma/\sigma_B$ for $\sigma_A/\sigma_B = 0.45$ and $\beta = 0.7$ at different $\alpha$ corresponding to $\alpha/\beta = 0.57$ (purple), 0.86 (green), 1.14 (cyan), 1.43 (orange) and 1.71 (yellow), from bottom to top. (b) $f_{\bar{\rm A}}$ (solid lines) and $f_{\bar{\rm B}}$ (dashed line) versus $\sigma/\sigma_{\rm B}$ for the same values of $\alpha/\beta$, from right to left.

## S2. CLASS 3C PHENOMENOLOGY

In the main article, we presented predictions for class 1 (thinning), class 3a (thinning then thickening) and class 3b (thickening then thinning) flow curves. Our model [using the functional forms of $f_{\bar{A}}(\sigma)$ and $f_{\bar{B}}(\sigma)$ given by Eq. (4-5)] also predicts two kinds of class 3c flow curve: "thins, thickens, thins", Fig. S2(a), and "thickens, thins, thickens", Fig. S2(b). The first type occurs when $\sigma_A/\sigma_B \gg 1$ and $\alpha/\beta > 1$ (i.e., type-$\mathcal{B}$ constraints are released more slowly with $\sigma$ than type-$\mathcal{A}$ ones are formed). Fig. S2(a) shows a representative set of flow curves for $\sigma_A/\sigma_B = 10$ at different values of $\alpha/\beta$. The re-entrant thinning is due to the continued release of type-$\mathcal{B}$ constraints after all type-$\mathcal{A}$ constraints have formed. The second type occurs for $\sigma_A/\sigma_B \sim 1$ whenever $\alpha/\beta$ is small. Figure S2(b) shows a series of representative flow curves at $\sigma_A/\sigma_B = 1$ and different $\alpha/\beta$ (see caption for parameters). For the set of parameters chosen, this type of flow curve emerges when $\alpha/\beta$ is below $\approx 0.5$. Fixing $\sigma_A/\sigma_B = 1$ and increasing $\alpha/\beta$ above 0.5 produces class 3b flow curves, which have a single viscosity peak and no subsequent trough.

While flow curves of the kind shown in Fig. S2(a) have been widely reported in the literature [1, 2], we are aware of no examples of the kind shown in Fig. S2(b).

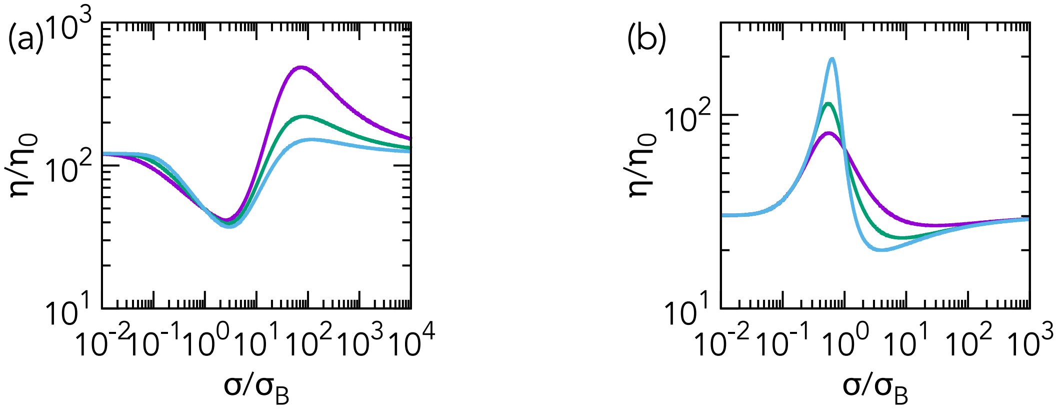


FIG. S2. Examples of class 3c flow curves for $\phi_{\bar{A}B} = \phi_{A\bar{B}} = 0.86\phi_{AB}$ and $\phi_{\bar{A}\bar{B}} = 0.47\phi_{AB}$. (a) "Thins, thickens, thins." Parameters, $\phi = 0.78\phi_{AB}$, $\sigma_A/\sigma_B = 10$, $\alpha = 1$ and different $\beta$ corresponding to $\alpha/\beta = 2.50$ (purple), 2.00 (green) and 1.67 (cyan). (b) "Thickens, thins, thickens." Parameters, $\phi = 0.70\phi_{AB}$, $\sigma_A/\sigma_B = 1$, $\alpha = 0.5$ and different $\beta$ corresponding to $\alpha/\beta = 0.50$ (purple), 0.33 (green) and 0.20 (cyan).

## S3. RELATIONSHIP BETWEEN FLOW CURVE CLASSES

In Fig. 1 of the main text, we presented examples of flow curves from classes 1, 3a and 3b. Here, we explore the relationship between them by systematically varying the ratio $\sigma_{\rm A}/\sigma_{\rm B}$, paying particular attention to the the various limiting viscosities. [Note also that in the main text, Fig. 1(a), (c) and (e) correspond to different $\phi$; here we compare different classes at the same $\phi$.]

Figure S3 plots relative viscosity $\eta/\eta_0$ as a function of $\sigma/\sigma_{\rm B}$ for $\alpha = \beta = 1$ at $\sigma_{\rm A}/\sigma_{\rm B} \to 0$ (purple), $\sigma_{\rm A}/\sigma_{\rm B} = 0.4$ (green), 1 (cyan), 10 (orange) and 100 (yellow). We chose all four jamming points to be different (in contrast to Fig. 1 of the main text, where $\phi_{\bar{\rm A}{\rm B}} = \phi_{{\rm A}\bar{\rm B}}$) to clearly highlight the relationships between the different classes. Specifically, we set $\phi_{\rm AB} = 0.64$, $\phi_{\bar{\rm A}\bar{\rm B}} = 0.30 = 0.47\phi_{\rm AB}$, $\phi_{\bar{\rm A}{\rm B}} = 0.55 = 0.86\phi_{\rm AB}$ and $\phi_{{\rm A}\bar{\rm B}} = 0.50 = 0.78\phi_{\rm AB}$. We present the predictions of our model at $\phi = 0.22 = 0.34\phi_{\rm AB}$.

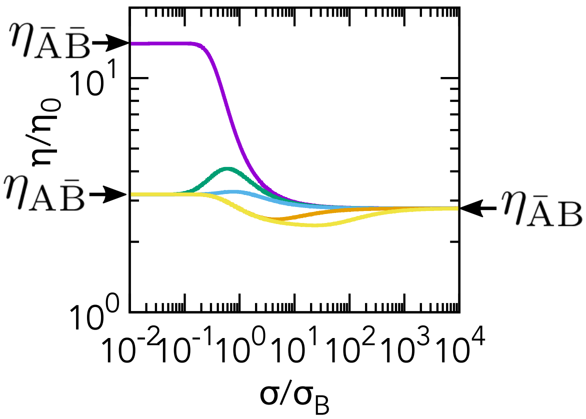


FIG. S3. Progression of flow curves as $\sigma_{\rm A}/\sigma_{\rm B}$ is increased for $\phi = 0.22 = 0.34\phi_{\rm AB}$. Lines denote relative viscosity $\eta/\eta_0$ as a function of $\sigma/\sigma_{\rm B}$ for $\alpha = \beta = 1$ and $\sigma_{\rm A}/\sigma_{\rm B} \to 0$ (purple), $\sigma_{\rm A}/\sigma_{\rm B} = 0.4$ (green), 1 (cyan), 10 (orange) and 100 (yellow). Jamming points, $\phi_{\rm AB} = 0.64$, $\phi_{\bar{\rm A}\bar{\rm B}} = 0.30 = 0.47\phi_{\rm AB}$, $\phi_{\bar{\rm A}{\rm B}} = 0.55 = 0.86\phi_{\rm AB}$ and $\phi_{{\rm A}\bar{\rm B}} = 0.50 = 0.78\phi_{\rm AB}$.

Consider the class 1 flow curve, $\sigma_{\rm A}/\sigma_{\rm B} \to 0$ (purple) in Fig. S3. Recall that for class 1, $\mathcal{A}$ is always constrained ($f_{\bar{\rm A}} = 1$) and thinning is driven by release of constraints on $\mathcal{B}$ [see Fig. 1(b) of the main text]. Thus, the viscosity shear thins from a low-$\sigma$ ($\sigma/\sigma_{\rm B} \ll 1$) plateau, $\eta_{\bar{\rm A}\bar{\rm B}}$, in which both $\mathcal{A}$ and $\mathcal{B}$ are constrained, to a high-$\sigma$ ($\sigma/\sigma_{\rm B} \gg 1$) plateau, $\eta_{\bar{\rm A}{\rm B}}$, in which only $\mathcal{A}$ is constrained. The plateau viscosities, $\eta_{\bar{\rm A}\bar{\rm B}}$ and $\eta_{\bar{\rm A}{\rm B}}$, are obtained by setting $\phi_{\rm J} = \phi_{\bar{\rm A}\bar{\rm B}}$ and $\phi_{\rm J} = \phi_{\bar{\rm A}{\rm B}}$ in Eq. (2), respectively. In general, $\eta_{\bar{\rm A}\bar{\rm B}} > \eta_{\bar{\rm A}{\rm B}}$. This is because $\eta$ increases

as the distance to jamming, $\phi_J - \phi$, decreases and the jamming point is lower in the more constrained state, $\phi_{\bar{A}\bar{B}} < \phi_{\bar{A}B}$.

Now consider the class 3a flow curve with $\sigma_A/\sigma_B = 100$ (yellow) in Fig. S3. Recall that for class 3a, the system initially shear thins as constraints on $\mathcal{B}$ are released while $\mathcal{A}$ is unconstrained, then, when constraints on $\mathcal{B}$ are removed, shear thickens as constraints on $\mathcal{A}$ are formed [see Fig. 1(d) of the main text]. Thus, the viscosity shear thins from a low-$\sigma$ plateau, $\eta_{A\bar{B}}$, in which only $\mathcal{B}$ is constrained, passes through a minimum, then shear thickens to a high-$\sigma$ plateau, $\eta_{\bar{A}B}$, in which only $\mathcal{A}$ is constrained. The relative values of $\eta_{A\bar{B}}$ and $\eta_{\bar{A}B}$ depend on the relative values of $\phi_{A\bar{B}}$ and $\phi_{\bar{A}B}$, and are not equal in general. (Note that $\eta_{A\bar{B}} = \eta_{\bar{A}B}$ in Fig. 1 of the main text only because we set $\phi_{A\bar{B}} = \phi_{\bar{A}B}$). For class 3b flow curves (green and cyan), which occur for $\sigma_A/\sigma_B \sim 1$, the viscosity shear thickens from $\eta_{A\bar{B}}$, reaches a peak, then shear thins to $\eta_{\bar{A}B}$.

There are two points of note. First, the limiting high-$\sigma$ viscosity is the same for all classes: there are only constraints on $\mathcal{A}$ in this limit and the viscosity equals $\eta_{\bar{A}B}$. Secondly, the low-$\sigma$ ($\sigma/\sigma_B \ll 1$) plateau viscosity is the same for class 3a and class 3b ($\eta_{A\bar{B}}$), but has a higher value for class 1 at the same $\phi$ ($\eta_{\bar{A}\bar{B}}$). This is because the prevailing contact state at low $\sigma$ for class 1, $\bar{A}\bar{B}$, involves more constraints than that for classes 3a and 3b, $A\bar{B}$. This difference also has important implications for the emergence of singular behavior, which we outline in §S5.

## S4. SINGULAR BEHAVIOR FOR CLASS 3

### A. Class 3a singular behavior: $\phi_{\mathrm{A\bar{B}}} = \phi_{\mathrm{\bar{A}B}}$ and $\phi_{\mathrm{A\bar{B}}} > \phi_{\mathrm{\bar{A}B}}$

In Fig. 3 of the main text, we examined the singular behavior of a class 3a system for $\phi_{\mathrm{A\bar{B}}} < \phi_{\mathrm{\bar{A}B}}$. We now examine the other two cases, $\phi_{\mathrm{A\bar{B}}} = \phi_{\mathrm{\bar{A}B}}$ and $\phi_{\mathrm{A\bar{B}}} > \phi_{\mathrm{\bar{A}B}}$.

Figure S4(a) shows a representative $\sigma$-$\phi$ phase diagram for $\phi_{\mathrm{\bar{A}B}} = \phi_{\mathrm{A\bar{B}}}$. The jamming boundary $\sigma_{\mathrm{jam}}(\phi)$ resembles Fig. 3(a) in the main text and tends to a point at $\phi_{\mathrm{max}} < \phi_{\mathrm{AB}} = \phi_{\mathrm{rcp}}$. Since $\phi_{\mathrm{\bar{A}B}} = \phi_{\mathrm{A\bar{B}}}$, $\phi_{\mathrm{jam}}(\phi)$ is never single valued: whenever the system yields at low $\sigma$, it subsequently re-jams at high $\sigma$. The jamming boundary for the other case, $\phi_{\mathrm{A\bar{B}}} > \phi_{\mathrm{\bar{A}B}}$, Fig. S4(b), is also similar to Fig. 3(a). It is double-valued for $\phi_{\mathrm{A\bar{B}}} < \phi < \phi_{\mathrm{max}}$, in which the system undergoes re-entrant jamming, and single-valued for $\phi_{\mathrm{\bar{A}B}} < \phi < \phi_{\mathrm{A\bar{B}}}$, in which the system flows at low $\sigma$ and jams at high $\sigma$. In all cases, there is also a region of unstable flow (gray) just below the jamming boundary $\sigma_{\mathrm{jam}}(\phi)$. For the parameters used in Fig. S4, the boundary of the unstable regime $\sigma_{\mathrm{uns}}(\phi)$ is slightly re-entrant and extends to $\phi < \phi_{\mathrm{\bar{A}B}}$.

*Comparison with Fall* et. al. *[3] in the main text*

In Fig. 3(b) of the main text, we compare flow curves predicted by our model to rheological data for suspensions of cornstarch in demineralised water from Ref. [3]. The authors of Ref. [3] do not report the viscosity of the suspending medium nor the temperature at which the measurements were performed; so, we take $\eta_0 = 1\,\mathrm{mPa\,s}$, the viscosity of water at 20 °C.

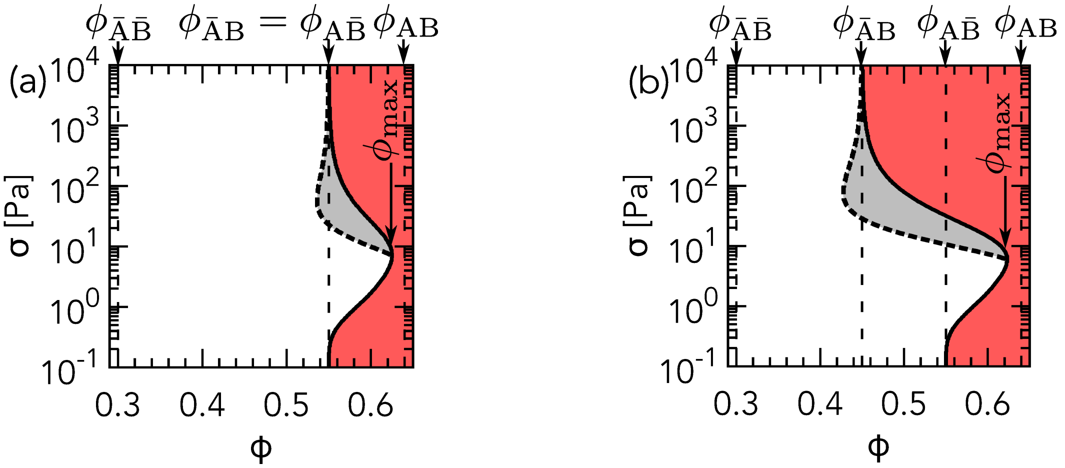


FIG. S4. Jamming phenomenology of class 3a. (a) $\sigma$-$\phi$ phase diagram for $\phi_{\bar{A}B} = \phi_{A\bar{B}}$ showing jammed (red), flowing (white) and unstable (gray) states. Solid curve, boundary of jammed states $\sigma_{jam}(\phi)$. Dashed curve, boundary of unstable states $\sigma_{uns}(\phi)$. Vertical dashed lines denote different jamming points, as labelled. Jamming points, $\phi_{AB} = 0.64$, $\phi_{\bar{A}B} = \phi_{A\bar{B}} = 0.55$ and $\phi_{\bar{A}\bar{B}} = 0.30$. Parameters, $\sigma_A = 25\,\mathrm{Pa}$, $\sigma_B = 1\,\mathrm{Pa}$ and $\alpha = \beta = 1$. (b) $\sigma$-$\phi$ phase diagram for $\phi_{\bar{A}B} < \phi_{A\bar{B}}$ with $\phi_{\bar{A}B} = 0.45$ and $\phi_{A\bar{B}} = 0.55$; other jamming points and parameters are the same as in (a).

### B. Class 3b singular behavior

Like class 3a, the $\sigma$-$\phi$ phase diagram for class 3b is rather complex and depends on the relative values of $\phi_{\bar{A}B}$ and $\phi_{A\bar{B}}$. We present an example with $\phi_{A\bar{B}} < \phi_{\bar{A}B}$ in Fig. S5(a) (see caption for parameters). $\sigma_{\rm jam}$ has a "nose" that extends to $\phi_{\rm nose} < \phi_{A\bar{B}}$, a characteristic feature of class 3b systems. Thus, for $\phi_{\rm nose} < \phi < \phi_{A\bar{B}}$ we predict re-entrant yielding, Fig. S5(b) (yellow and black curves): the system flows at low $\sigma$, shear-jams when $\sigma$ reaches the lower part of $\sigma_{\rm jam}$, then un-jams (yields) when $\sigma$ crosses the upper boundary. At $\phi = \phi_{A\bar{B}}$, the low-$\sigma$ shear-jamming regime vanishes, Fig. S5(b) (blue and red curves), and the system simply has a yield stress $\sigma_{\rm y}(\phi)$ that diverges at $\phi_{\bar{A}B} > \phi_{A\bar{B}}$. There is also a region of $\sigma$-$\phi$ space [grey in Fig. S5(a)] in which we predict unstable flow.

The transition from peaked $\eta(\sigma)$ to yield stress behavior with increasing $\phi$ is consistent with the experimental observations in Ref. [4]. Experiments have yet to probe the re-entrant yielding regime fully. If the behavior shown in Fig. S5 is found in an experimental system, it will be a strong argument for the applicability of our two-constraint picture.

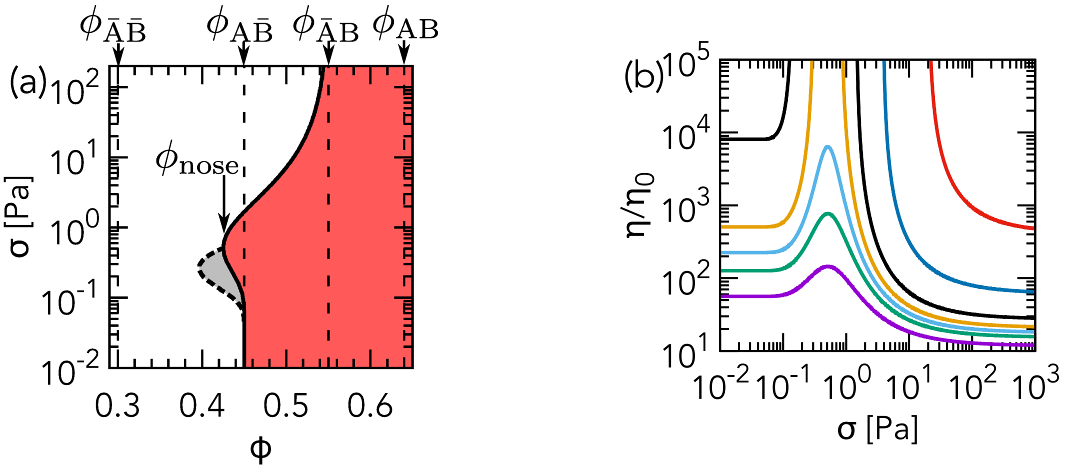


FIG. S5. Jamming phenomenology for class 3b. Jamming points, $\phi_{AB} = 0.64$, $\phi_{\bar{A}B} = 0.55$, $\phi_{A\bar{B}} = 0.45$ and $\phi_{\bar{A}\bar{B}} = 0.30$. Model parameters, $\sigma_A = 0.4\,$Pa, $\sigma_B = 1\,$Pa, $\alpha = 1$, $\beta = 0.7$. (a) $\sigma$-$\phi$ phase diagram. (b) $\eta/\eta_0$ versus $\sigma/\sigma_B$ at $\phi = 0.39$ (purple), 0.41 (green), 0.42 (cyan), 0.43 (yellow), 0.445 (black), 0.48 (blue) and 0.523 (red), from bottom to top.

## S5. COMPARISON OF JAMMING PHASE DIAGRAMS

In this section, we briefly compare class 1 and class 3a singular behavior and comment on the interpretation of experimental data that is available in a restricted $\sigma$-window.

### A. Emergence of a yield stress in classes 1 and 3a

A full discussion of the physics behind the $\sigma$-$\phi$ phase diagrams in Fig. 2(a) and 3(a), including the precise form of the jamming boundary, $\sigma_{\mathrm{jam}}(\phi)$, is beyond the scope of the current work. However, the volume fraction at which the system develops a non-zero yield stress can be readily deduced. Class 1 systems, Fig. 2(a), develop a yield stress when the class-1, low-$\sigma$ plateau viscosity, $\eta_{\bar{\mathrm{A}}\bar{\mathrm{B}}}(\phi) \equiv (1 - \phi/\phi_{\bar{\mathrm{A}}\bar{\mathrm{B}}})^{-2}$ (Fig. S3), diverges, i.e, at $\phi = \phi_{\bar{\mathrm{A}}\bar{\mathrm{B}}}$. Class 3a systems, Fig. 3(a), develop a yield stress at a higher concentration, $\phi_{\mathrm{A}\bar{\mathrm{B}}}$, where the class-3a, low-$\sigma$ plateau viscosity, $\eta_{\mathrm{A}\bar{\mathrm{B}}}(\phi) = (1 - \phi/\phi_{\mathrm{A}\bar{\mathrm{B}}})^{-2}$, diverges. This difference arises because class 1 systems are more constrained than class 3a systems in the $\sigma/\sigma_{\mathrm{B}} \ll 1$ limit, as discussed in §S3.

### B. Interpretation of limited experimental data

In experiments, one can observe the rheology only in a finite $\sigma$-window, determined, e.g., by the torque resolution of the rheometer at low $\sigma$ and edge fracture at high $\sigma$ [5]. Thus, in some cases, it may not be possible to deduce the “true” class of flow curve (1, 2, 3a etc.) based on a measurement at a single $\phi$. For example, consider a system whose “true” behavior is class 3a, i.e., thinning followed by thickening, Fig. S6(a) (solid curve), but for which only the shear-thinning section is visible due to the experimental $\sigma$-window (shaded gray). Based on a single flow curve, it would be impossible to distinguish this scenario from the one schematized in Fig. S6(b), in which the underlying behavior is class 1.

Despite the topological similarity between the observable $\eta(\sigma)$ in Fig. S6(a) and (b), the underlying constraint physics is distinct, as discussed in §S3. The difference would be revealed only by mapping out the full $\sigma$-$\phi$ phase diagram, as in Fig. 2(a) or 3(a). In this particular example, the emergence of a yield stress at $\phi_{\mathrm{A}\bar{\mathrm{B}}}$ would indicate scenario (a) (class 3a); whereas, the emergence of a yield stress at $\phi_{\bar{\mathrm{A}}\bar{\mathrm{B}}}$ ($< \phi_{\mathrm{A}\bar{\mathrm{B}}}$) would indicate scenario (b)

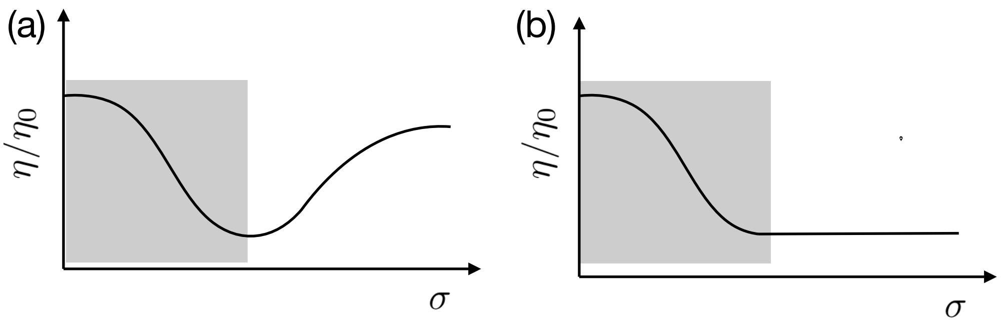


FIG. S6. Schematic flow curves for (a) class 3a and (b) class 1 systems. Only the $\sigma$ range inside the gray-shaded window is visible experimentally. Despite the topological similarity of the curves in the visible window, the underlying constraint physics is distinct.

(class 1).

[1] E. Bertrand, J. Bibette, and V. Schmitt, Phys. Rev. E **66**, 060401 (2002).

[2] S. Jamali, A. Boromand, N. Wagner, and J. Maia, J. Rheol. **59**, 1377 (2015).

[3] A. Fall, F. Bertrand, D. Hautemayou, C. Mézière, P. Moucheront, A. Lemaitre, and G. Ovarlez, Phys. Rev. Lett. **114**, 098301 (2015).

[4] S.-C. Dai, E. Bertevas, F. Qi, and R. I. Tanner, J. Rheol. **57**, 493 (2013).

[5] B. M. Guy, M. Hermes, and W. C. K. Poon, Phys. Rev. Lett. **115**, 088304 (2015).
